# Supplementary material for: Finite-time Non-overshooting Leader-following Consensus Control for Multi-Agent Systems
Source: arXiv:2412.07855 source file (2024-12-10)
Supplement: Supplementary file 1 [file VI_Appendix.tex]

\section*{Appendix}
